# Supplementary material for: Crossing Variational Autoencoders for Answer Retrieval
Source: arXiv:2005.02557 source file (2020-07-06)
Supplement: Supplementary file 1 [file appendix.tex]

\subsection{Dataset}
SQuAD 1.1 is a reading comprehension challenge
that consists of over 100,000 questions composed to be answerable by text from Wikipedia articles. The data is organized into paragraphs, where each paragraph has multiple associated questions. Each question can have one or more answers in its paragraph.

\subsection{Baselines}

Dual encoder models are learned functions that collocate queries and results in a shared embedding space. This architecture has shown strong performance on sentence-level retrieval tasks, including conversational response retrieval \cite{yang2018learning,henderson2017efficient}, translation pair retrieval \cite{guo2018effective,yang2019improving} and similar text retrieval \cite{gillick2018end}.

\vspace{0.1in}
\noindent\textbf{USE-QA.} As our primary neural baseline, we take the recently released universal sentence encoder QA (USE-QA) \cite{yang2019multilingual}. This
is a multilingual QA retrieval model that co-trains a question-answer dual encoder along with secondary tasks of translation ranking and natural language inference. The model uses sub-word tokenization, with a 128k “sentencepiece” vocabulary \cite{kudo2018sentencepiece}. Question and
answer text are encoded independently using a 6-layer transformer encoder \cite{vaswani2017attention}, and then reduced to a fixed-length vector through average pooling. The final encoding dimensionality is 512. The training corpus contains over a billion question-answer pairs from popular online forums and QA websites like Reddit and StackOverflow. Codes are published by Google, which could be downloaded at \url{https://tfhub.dev/google/universalsentence-encoder-multi\\lingual-qa/1}

\vspace{0.1in}
\noindent\textbf{QA-Lite.} As a second neural baseline, we include an internal QA model (QA-Lite) designed for use on mobile devices. Like USE-QA, this model is trained over online forum data, and uses a transformer based text encoder. The core differences are reduction in width and depth of model layers, reduction of sub-word vocabulary size, and a decrease in the output embedding size from 512 dimensions to only 100.

\noindent\textbf{InferSent.} Finally, we include the text embedding system InferSent, which, although not explicitly designed for question answering tasks\footnote{The non-QA versions of the Universal Sentence Encoder produce general semantic embeddings of text.}, nevertheless produces strong results on a wide range of semantic tasks without requiring additional fine tuning \cite{conneau2017supervised}.

\begin{table}[t]
\centering
\caption{The details and statistical results of datasets.}
\label{tab:Dataset-detail-BioNER}
\vspace{-0.1in}
{\scalebox{0.7}{%
\begin{tabular}{l|cccc|ccc}
\toprule
\multirow{2}{*}{\textbf{Dataset}} & \multicolumn{4}{l|}{\textbf{\# sentences}} & \multicolumn{2}{l}{\textbf{\# lengths}} \\
 & train & dev & test & total & QL & AL & Vocab\\ \hline
\textbf{SQuAD} & 87599 & 11246 & N/A & 98845 & 11.18 & 31.44 & 113,649\\
\textbf{Lenovo} & 10369 & 1278 & 2573 & 12942 & 54.75 & 38.99 & 23,072\\
\textbf{AskUbuntu} & 43748 & 4872 & 9797 & 58417 & 45.28 & 32.70 & 57,982 \\
\bottomrule

\end{tabular}}}
\end{table}

\begin{table}[t]
\centering
\caption{The details and statistical results of datasets.}
\label{tab:Dataset-detail-BioNER}
\vspace{-0.1in}
{\scalebox{0.7}{%
\begin{tabular}{l|cc|cc}
\toprule
\multirow{2}{*}{\textbf{Dataset}} & \multicolumn{2}{l|}{\textbf{\# Drop StopWord}} & \multicolumn{2}{l}{\textbf{\# With StopWord}} \\
 & QinA & AinQ & QinA & AinQ  \\ \hline
\textbf{SQuAD} & 44.15(23.0) & 18.69(14.0) & 44.97(19.4) & 23.81(14.8) \\
\textbf{SQuAD(p)} & 54.71(19.5) & 10.40(6.96) & 57.42(16.4) & 16.28(8.52)  \\
\textbf{Lenovo} & 12.42(11.7) & 16.15(12.49) & 23.63(13.2) & 30.59(13.83)  \\
\bottomrule

\end{tabular}}}
\end{table}

\subsection{Implementation Details}

% \begin{table}[t]
% \caption{Performance of question answering retrieval on SQuAD dataset by different methods, where ``*'' indicates result reproduced by open tools.}
% \label{tab:Baseline-BioNER-different-corpus}
% \scalebox{0.88}{%
% \setlength{\tabcolsep}{1.2mm}{
% \begin{tabular}{llllll}
% \toprule
% \multicolumn{1}{c}{Models} & MRR & R@1 & R@5 & R@10 & R@50 \\ \hline
% \textbf{QA-Lite(Google)*}  & - & - & - & - & - \\
% % \textbf{BERT-QA*}  & 37.57 & 31.10 & 44.39 & 50.20 & 63.89  \\
% \textbf{ReQA(Google)*}  & 59.18 & 51.26 & 68.33 &\textbf{ 75.29} &\textbf{ 88.27 }\\
% \textbf{BERT-VAE} & 59.94 & 53.72 & 67.21 & 72.53 & 84.09 \\
% \textbf{BERT-CAVAE}  & \textbf{61.39} &\textbf{ 55.02} &\textbf{ 68.66 }& 74.28 & 85.55
% \bottomrule
% \end{tabular}}}
% \end{table}

\begin{table*}[]
\centering
\caption{Performance of question answering retrieval on Lenovo dataset by different methods, where ``*'' indicates result reproduced by open tools.}
\label{tab:stoa-result}
\scalebox{0.7}{%
\begin{tabular}{l|ccccc|ccccc|ccccc}
\toprule
\multirow{2}{*}{\textbf{Method}} & \multicolumn{5}{c}{\textbf{SQuAD}} & \multicolumn{5}{c}{\textbf{Lenovo}} & \multicolumn{5}{c}{\textbf{AskUbuntu}} \\
 & MRR & R@1 & R@5 & R@10 & R@50 & MRR & R@1 & R@5 & R@10 & R@50 & MRR & R@1 & R@5 & R@10 & R@50 \\ \hline
\textbf{InferSent*}  & - & - & - & - & - & - & - & - & - & - & - & - & - & - & - \\
\textbf{QA-Lite*} & - & - & - & - & - & - & - & - & - & - & - & - & - & - & - \\
\textbf{BERT-Share*} & 49.09 & 44.15 & 54.38 & 59.35 & 70.73 & - & - & - & - & - & - & - & - & - & - \\
\textbf{BERT-Dual} & 56.25 & 50.44 & 62.78 & 68.27 & 80.15 & - & - & - & - & - & - & - & - & - & - \\
\textbf{ReQA(Google)*}  & 59.18 & 51.26 & 68.33 &\textbf{ 75.29} &\textbf{ 88.27 } & - & - & - & - & - & - & - & - & - & -  \\
\textbf{LSTM-CAVAE}  & \textbf{61.39} &\textbf{ 55.02} &\textbf{ 68.66 }& 74.28 & 85.55 & - & - & - & - & - & - & - & - & - & - \\
\textbf{BERT-CAVAE} & - & - & - & - & - & - & - & - & - & - & - & - & - & - & - \\
\bottomrule
\end{tabular}}
\end{table*}

% & 18.02 & 11.74 & 23.40 & 30.27 & 49.83
\begin{table*}[]
\centering
\caption{Performance of question answering retrieval on Lenovo dataset by different methods, where ``*'' indicates result reproduced by open tools.}
\label{tab:stoa-result}
\scalebox{0.7}{%
\begin{tabular}{l|ccccc|ccccc|ccccc}
\toprule
\multirow{2}{*}{\textbf{Method}} & \multicolumn{5}{c}{\textbf{SQuAD}} & \multicolumn{5}{c}{\textbf{Lenovo}} & \multicolumn{5}{c}{\textbf{AskUbuntu}} \\
 & MRR & R@1 & R@5 & R@10 & R@50 & MRR & R@1 & R@5 & R@10 & R@50 & MRR & R@1 & R@5 & R@10 & R@50 \\ \hline
\textbf{LSTM-Dual} & 58.11 & 52.16 & 64.78 & 70.32 & 82.18 & 8.93 & 6.06 & 11.08 & 14.42 & 23.05 & - & - & - & - & -  \\
\textbf{LSTM-VAE} & 60.01 & 53.60 & 67.49 & 72.63 & 84.29 & - & - & - & - & -  & - & - & - & - & - \\
\textbf{LSTM-CVAE}  & 60.62 & 54.30 & 67.85 & 73.40 & 84.85 & - & - & - & - & - & - & - & - & - & - \\
\textbf{LSTM-CAVAE}  & \textbf{61.43} &\textbf{ 55.04} &\textbf{ 68.72 }& \textbf{74.28} & \textbf{85.55} & 11.57 & 7.27 & 14.55 & 20.02 & 37.11 & - & - & - & - & - \\
\textbf{BERT-Dual} & - & - & - & - & - & - & - & - & - & - & - & - & - & - & -  \\
\textbf{BERT-VAE} & - & - & - & - & - & - & - & - & - & - & - & - & - & - & - \\
\textbf{BERT-CVAE}  & - & - & - & - & - & - & - & - & - & - & - & - & - & - & - \\
\textbf{BERT-CAVAE} & - & - & - & - & - & - & - & - & - & - & - & - & - & - & - \\
\bottomrule
\end{tabular}}
\end{table*}

    % Recall@1 on test is 0.5542
    % Recall@5 on test is 0.6892
    % Recall@10 on test is 0.7462
    % Recall@200 on test is 0.9294
    % MRR on test is 0.6174

% \\
% (1) SQuAD test? \\
% (2) Context -. Long/MRR \\
% 1. No contextual information in question and answer. 
% 2. Long / Not same space.

% (3) QA alignment \\
% (4) VAE \\

>10
Recall@1 is 0.35537190082644626
Recall@5 is 0.4793388429752066
Recall@10 is 0.5785123966942148
Recall@50 is 0.8099173553719008
mrr 0.4275142360968425

BERT
Recall@1 on testsub is 0.2810 
Recall@5 on testsub is 0.3306 
Recall@10 on testsub is 0.3554 
Recall@50 on testsub is 0.4793 
MRR on testsub is 0.3093

>16
Recall@1 is 0.23529411764705882
Recall@5 is 0.29411764705882354
Recall@10 is 0.29411764705882354
Recall@50 is 0.7058823529411765
mrr 0.2774411679183268

\subsection{Experimental Results}

\subsection{Case Study}

\begin{table}[]
\centering
\caption{Performance of question answering retrieval on Lenovo dataset by different methods, where ``*'' indicates result reproduced by open tools.}
\label{tab:stoa-result}
\scalebox{0.85}{%
\begin{tabular}{lccccc}
\toprule
\multirow{2}{*}{\textbf{Method}} & \multicolumn{5}{c}{\textbf{SQuAD}} \\
 & MRR & SSE & R@1 & R@5 & R@10  \\ \hline
\textbf{$\bf {BERT}_{QA}$} & 58.11 & 52.16 & 64.78 & 70.32 & 82.18  \\
\textbf{USE-QA} & 58.11 & 52.16 & 64.78 & 70.32 & 82.18  \\
\textbf{CAVAE} & 42.62 & - & 38.84 & 44.63 & 52.89  \\
\bottomrule
\end{tabular}}
\end{table}

Recall@1 on testsub is 0.3884
Recall@5 on testsub is 0.4463
Recall@10 on testsub is 0.5289
Recall@200 on testsub is 0.8678
MRR on testsub is 0.4262

Recall@1 on testsub is 0.4050
Recall@5 on testsub is 0.4463
Recall@10 on testsub is 0.5289
Recall@200 on testsub is 0.8595
MRR on testsub is 0.4390
